# Supplementary material for: BER-Based Physical Layer Security with Finite Codelength: Combining Strong Converse and Error Amplification
Source: arXiv:1412.5227 source file (2015-01-04)
Supplement: Supplementary file 1 [file additional_A.tex]

\clearpage
\newpage
\section{Security Gap for GI-AWGN when $R \rightarrow \infty$}

{\it Corollary 1:} When $0< {\cal P}_\err^{\bob,\Th} <1$ and $0<{\cal P}_\err^{\eve,\Th} < 1$, the security gap is asymptotically given by \beqa \lim_{n \rightarrow \infty} \Delta S &=& 0  \\   \lim_{R \rightarrow \infty}\Delta S &=& 10 \log_{10} \frac{ (1 + \breve \rho_\infty) \left( {\cal P}_\err^{\bob,\Th} \right)^{-\frac{1}{n \breve \rho_\infty}}  }{(1+\breve \rho'_\infty)\left(1- {\cal P}_\err^{\eve,\Th} \right)^{-\frac{1}{n \breve \rho'_\infty}} }  \eeqa
where \beqa \breve \rho_\infty &=& \frac{1}{2} \left( \ln u_\bob + \left((\ln u_\bob)^2 + 4 \ln u_\bob \right)^{\frac{1}{2}} \right) \\  \breve \rho'_\infty &=& \frac{1}{2} \left(\ln u_\eve - \left((\ln u_\eve)^2 + 4 \ln u_\eve \right)^{\frac{1}{2}} \right) \eeqa
where $u_\bob = ({\cal P}_\err^{\bob,\Th})^{- \frac{1}{n} }$ and $u_\eve = (1-{\cal P}_\err^{\eve,\Th})^{- \frac{1}{n} }$.

{\it Proof:} As $n \rightarrow \infty$, we have $\min_{0 < \rho \leq 1} g_\bob(\rho) \rightarrow  (e^R-1)$ and $\max_{-1 < \rho' <0} g_\bob(\rho) \rightarrow (e^R-1)$, and thus, $\Delta S \rightarrow 0$. Also,
\beqa \lim_{R \rightarrow \infty} \Delta S &=& 10 \log_{10} \left( \lim_{R \rightarrow \infty} \frac{\min_{0 < \rho \leq 1} g_\bob(\rho)} {\min_{-1 < \rho' < 0} g_\eve(\rho')} \right) \\ &=& 10 \log_{10} \left( \lim_{R \rightarrow \infty} \frac{ g_\bob(\breve \rho_\infty)}{g_\eve(\breve \rho'_\infty)} \right). \eeqa In the above,
\beqa \breve \rho_\infty &=& \arg \lim_{R \rightarrow \infty} \min_{0 < \rho \leq 1} g_\bob(\rho) \\ &\stackrel{(a)}{=}&{\rm sol}_{\rho} \left\{ \lim_{R \rightarrow \infty} \frac{\partial }{\partial \rho} g_\bob(\rho)=0 \right\}  \\ \breve \rho'_\infty &=& \arg \lim_{R \rightarrow \infty} \min_{-1 < \rho' < 0} g_\eve(\rho') \\ &\stackrel{(b)}{=}& {\rm sol}_{\rho'} \left\{ \lim_{R \rightarrow \infty} \frac{\partial }{\partial \rho'} g_\eve(\rho')=0 \right\} \eeqa where ${\rm sol}_\alpha \{ f(\alpha) =0 \}$ denotes the solution to $f(\alpha) =0$. Note that $(a)$ holds only when the solution to $\lim_{R \rightarrow \infty} \frac{\partial }{\partial \rho} g_\bob(\rho)=0$ exist and it is unique. The same for $(b)$.
From \beq \lim_{R \rightarrow \infty} \frac{\partial }{\partial \rho} g_\bob(\rho) =\lim_{R \rightarrow \infty} \left\{ u_\bob^{\frac{1}{\rho}} e^R-1 + (1+\rho) \left( -\frac{1}{\rho^2} u_\bob^{\frac{1}{\rho}} e^R \ln u_\bob -1 \right) \right\} = 0\eeq we have \beq  u_\bob^{\frac{1}{\rho}}  - (1+\rho) \frac{1}{\rho^2} u_\bob^{\frac{1}{\rho}} \ln u_\bob   = 0\eeq There exists a unique valid solution to $\lim_{R \rightarrow \infty} \frac{\partial }{\partial \rho} g_\bob(\rho)=0$ and it is given by $\breve \rho_\infty =\frac{1}{2} \left( \ln u_\bob + \left((\ln u_\bob)^2 + 4 \ln u_\bob \right)^{\frac{1}{2}}\right)$. In the same way, one can show that there exist a unique solution to $\lim_{R \rightarrow \infty} \frac{\partial }{\partial \rho'} g_\eve(\rho')=0$ and it is given by $\breve \rho'_\infty =\frac{1}{2} \left( \ln u_\eve - \left((\ln u_\eve)^2 + 4 \ln u_\eve \right)^{\frac{1}{2}} \right)$.

\hfill $\Box$

(Question:) The range of $\breve \rho_\infty$ and $\breve \rho'_\infty$ must be \beqa 0 < \breve \rho_\infty \leq 1 \\ -1 < \breve \rho'_\infty < 0 \eeqa

How can we ensure this???

\clearpage
\newpage
\section{Security Gap for BSC}

{\it Remark:} Although the security gap was originally considered only for AWGN channels, the concept can be extended to other channels such as BSC and BEC. Let $\delta_\bob$ denote the crossover and erasure probabilities for BSC and BEC, respectively, for Bob. For BEC, we have \beqa E_0^\bob(\rho,q_{\rm uni}(x),\delta_\bob) &=& -\ln \left[ 2^{-\rho} (1-\delta_\bob) +\delta_\bob \right] \\ E_0^\eve(\rho',q_{\rm uni}(x),\delta_\eve) &=& -\ln \left[ 2^{-\rho'} (1-\delta_\eve) +\delta_\eve \right]  \eeqa For BSC, we have \beqa E_0^\bob(\rho,q_{\rm uni}(x),\delta_\bob) &=& -\ln \left[ 2^{-\rho} \left( \delta_\bob^{\frac{1}{1+\rho}}+(1-\delta_\bob)^{\frac{1}{1+\rho}} \right)^{1+\rho} \right] \\ E_0^\eve(\rho',q_{\rm uni}(x),\delta_\eve) &=& -\ln \left[ 2^{-\rho'} \left( \delta_\eve^{\frac{1}{1+\rho'}}+(1-\delta_\eve)^{\frac{1}{1+\rho'}} \right)^{1+\rho'} \right] \eeqa

The BER bounds are given by \beqa P_\ber^{\bob,\up}(R,\rho, \delta_\bob) &=& 0.5 \exp \left( -n \left\{ E_0^\bob(\rho,q_{\rm uni}(x),\delta_\bob)-\rho R \right\} \right) \\ P_\ber^{\eve,\low}(R,\rho', \delta_\eve) &=& P_\ber^{\rm SPN, \low}(r,K)\cdot \left( 1- \exp \left( -n \left\{ E_0^\eve(\rho',q_{\rm uni}(x),\delta_\eve)-\rho' R  \right\} \right) \right) \eeqa

Then an upper-bound of the security gap can be defined as the difference between the two probabilities as follows:
\beqa && \Delta S_\up  :=  \delta_{\eve,\up}^{\min} - \delta_{\bob,\low}^{\max} \eeqa where $\delta_\bob^{\max}$ and $\delta_\eve^{\min}$ are determined by \beqa \delta_{\bob,\low}^{\max}= \max \delta_\bob {\rm ~~~subject ~ to ~~~}  P_\ber^{\bob, \low}(R,\breve \rho,\delta_\bob) \leq \calP_\ber^{\bob,\Th} \\ \delta_{\eve,\up}^{\min}= \min \delta_\eve  {\rm ~~~subject ~ to ~~~} P_\ber^{\eve, \up}(R,\breve \rho', \delta_\eve) \geq \calP_\ber^{\eve,\Th}  \eeqa
where $\breve \rho$ is optimal $\rho$ minimizing $P_\ber^{\bob,\up}(R, \rho,\delta_\bob)$ and $\breve \rho'$ is optimal $\rho'$ maximizing $P_\ber^{\eve,\low}(R, \rho',\delta_\eve)$.

{\it Theorem 2:} $\delta_\bob^{\max}$ and $\delta_\eve^{\min}$ are \beqa \delta_\bob^{\max}(\rho) &=&  (1-2^{-\rho})^{-1} \left\{ \left(\varepsilon_\ber^{\bob,\Th} \right)^{\frac{1}{n}} e^{-\rho R} - 2^{-\rho} \right\} \\ \delta_\eve^{\min}(\rho') &=&  (1-2^{-\rho'})^{-1} \left\{ \left(\varepsilon_\ber^{\eve,\Th} \right)^{\frac{1}{n}} e^{-\rho' R} - 2^{-\rho'} \right\}
\\ \tilde \rho &=&\arg \max_{0 < \rho \leq 1}  \delta_\bob^{\max} (\rho) \label{eq:optimization_rho_1} \\ \tilde \rho' &=& \arg \min_{-1< \rho' <0}  \delta_\eve^{\min} (\rho'). \label{eq:optimization_rho_prime_1}  \eeqa

(Question:) We didn't get reasonable numerical results???

\clearpage
\newpage
\section{Outage probability when ${\cal P}_\err^{\eve,\Th} \rightarrow 0$. }

When ${\cal P}_\err^{\eve,\Th} \rightarrow 0$ (that is, with $no$ the security condition), the maximum power $p_{\max}(\Gamma_\eve, \rho') \rightarrow \infty$. Therefore, the overall outage probability must decrease indefinitely with $p_\av/\sigma^2$ with no error floor, as in the conventional outage probability of Caire's paper.

In my approach, however, we still have a error floor even when ${\cal P}_\err^{\eve,\Th} \rightarrow 0$. Please see the figure. The reason is as follows. No matter what the value of ${\cal P}_\err^{\eve,\Th}$, the maximum power $p_{\max}(\Gamma_\eve, \rho')$ is upper-limited by $p_0$, where $C_\eve = \ln(1 + p_0)$, because we use Eve's error lower-bound equation, which is valid only when $R> C_\eve$. Overall, even when ${\cal P}_\err^{\eve,\Th} \rightarrow 0$, we still have an error floor.

In the numerical results, the error floor is independent of ${\cal P}_\err^{\eve,\Th}$.

\begin{figure}[h]
\begin{center}
\includegraphics[width=1.1\columnwidth]{figure/Additional/additional_1}
\caption{Overall outage probability floor}
\label{fig:additional_1}
\end{center}
\end{figure}

\begin{figure}[h]
\begin{center}
\includegraphics[width=0.7\columnwidth]{figure/Additional/additional_2}
\caption{Overall outage probability floor}
\label{fig:additional_2}
\end{center}
\end{figure}

\clearpage
\newpage
\section{Minimization of Bob's Average BER subject to Security Constraint}

In this subsection, another approach is considered to optimize the transmit power. Taking expectation over $\gamma_\bob$, we first define Bob's average BER upper-bound as follows: \beqa \bar P_\ber^{\bob,\up}(R):&=& \mathbb{E} \left[ P_\ber^{\bob,\up}(R, \rho(\gamma_\bob),\gamma_\bob) \right], ~~~0< \rho \leq 1 \\ &=& 0.5 \mathbb{E} \left[ \exp \left( -n  \left\{  -\ln \left( 1+ \frac{ p \gamma_\bob  }{ (1+\rho(\gamma_\bob))  } \right)^{-\rho(\gamma_\bob)}  - \rho(\gamma_\bob) R \right\} \right) \right]. \label{eq:avg Bob_BER_Gau}    \eeqa
The transmit power is optimized to minimize $\bar P_\ber^{\bob,\up}(R)$ subject to a security constraint constraining Eve's instantaneous BER to be greater than a threshold as follows:
\begin{subequations}
\beqa && \min_{p(\gamma_\bob, \gamma_\eve),0< \rho(\gamma_\bob) \leq 1,-1< \rho'(\gamma_\eve)<0} \bar P_\ber^{\bob,\up}(R) \\ && {\rm subject ~ to} ~   p(\gamma_\bob, \gamma_\eve) \geq 0\\ && \hspace{1.9cm} \mathbb{E}[p(\gamma_\bob, \gamma_\eve)] \leq p_\av \\ && \hspace{1.9cm}  P_\ber^{\eve,\low}(R,\rho'(\gamma_\eve),\gamma_\eve) \geq \calP_\ber^{\eve,\Th}.\label{eq:prob_2_opt_1_constraint_3}  \eeqa \label{eq:prob_2_opt_1}   \end{subequations}
In the following, the optimal solution is derived.

{\it Theorem 2:} The optimal solution to (\ref{eq:prob_2_opt_1}) is given by
\beq p_{\opt 2}(\gamma_\bob, \gamma_\eve) = \min \left(p_\opt^{\bob,\up}(\gamma_\bob,\hat \rho,\lambda), p_{\max}(\gamma_\eve,\tilde \rho')  \right) \label{eq:p_opt2} \eeq
where $p_{\max}(\gamma_\eve, \rho')$ is given by (\ref{eq:p_max_Eve}) and   $p_\opt^{\bob,\up}(\gamma_\bob,\rho,\lambda)$ is given by
\beq p_\opt^{\bob,\up}(\gamma_\bob,\rho,\lambda) = \left( \left(\frac{\lambda \gamma_\bob^{\rho}}{ \rho (1+  \rho)^{  \rho} }\right)^{-\frac{1}{  \rho+1}} - \frac{1+ \rho}{\gamma_\bob} \right)^+. \label{eq:p_opt_b_u} \eeq
In (\ref{eq:p_opt2}), $\tilde \rho'$ is determined by (\ref{eq:optimization_rho_prime_1}) and then $\hat \rho(\gamma_\bob)$ is determined by
\beqa \hat \rho(\gamma_\bob) &=& \arg \max_{0<\rho(\gamma_\bob) \leq 1}  \left\{ E_0^\bob \left(\rho(\gamma_\bob),{\cal CN}\left(0,\min\left(p_\opt^{\bob,\up}(\gamma_\bob,\rho (\gamma_\bob),\lambda), p_{\max}(\gamma_\eve,\tilde \rho')  \right) \right),\gamma_\bob\right) - \rho(\gamma_\bob) R \right\} \non \\
\\ &=& \arg \max_{0<\rho(\gamma_\bob) \leq 1}  \left\{ -\ln \left( 1+ \frac{ \min \left(p_\opt^{\bob,\up}(\gamma_\bob, \rho(\gamma_\bob),\lambda), p_{\max}(\gamma_\eve, \tilde \rho')  \right) \gamma_\bob  }{1+\rho(\gamma_\bob)} \right)^{-\rho(\gamma_\bob)} - \rho(\gamma_\bob) R \right\} \non \\ \label{eq:optimizatio_hat_rho} \eeqa where the optimal $\hat \rho(\gamma_\bob)$ always exists and $\lambda$ is determined such that the following condition is satisfied:\beqa \mathbb{E} [  p_{\opt 2}(\gamma_\bob, \gamma_\eve)]= p_\av . \eeqa

{\it Proof of Theorem 2:} See Appendix B. \hfill $\Box$

Note that the exponent is positive: \beq E_0^\bob \left(\hat\rho(\gamma_\bob),{\cal CN}\left(0,p_{\opt 2}( \gamma_\bob,\gamma_\eve)  \right),\gamma_\bob\right) - \hat \rho(\gamma_\bob) R>0, ~~~~ R< C_\bob(\gamma_\bob,\gamma_\eve) \eeq where $C_\bob(\gamma_\bob,\gamma_\eve)$ is time-varying given by \beq C_\bob(\gamma_\bob,\gamma_\eve) = \ln \left(1+ \min \left(p_\opt^{\bob,\up}(\gamma_\bob,\hat \rho,\lambda), p_{\max}(\gamma_\eve,\tilde \rho')\right) \gamma_\bob \right) \eeq

(Problem): Depending on $\gamma_\bob$ and $\gamma_\eve$, the following situation happens \beq R > C_\bob(\gamma_\bob, \gamma_\eve) \eeq In this case, $E_0^\bob(\cdot) < 0$ and the corresponding instantaneous BER is 0.5, which makes the average BER not very small even when all other instantaneous BERs are extremely small.

In particular, when $p_\av \rightarrow \infty$, we have $p_\opt^{\bob,\up}(\gamma_\bob,\hat \rho,\lambda) \rightarrow \infty$; but $p_{\max}(\cdot)$ is not affected by $p_\av$. Therefore, the capacity is bounded by $p_{\max}(\cdot)$: \beqa C_\bob(\gamma_\bob, \gamma_\eve) & \leq & \ln \left(1+  p_{\max}(\gamma_\eve,\tilde \rho') \gamma_\bob \right) \\ & =: & C'_\bob(\gamma_\bob,\gamma_\eve) \eeqa Note that $C'_\bob(\gamma_\bob,\gamma_\eve)$ is time-varying and it is very possible: \beq R > C'_\bob(\gamma_\bob, \gamma_\eve) \eeq

\newpage

We now assume that $\rho$ is a constant that is independent of $\gamma_\bob$. Taking expectation over $\gamma_\bob$, we first define Bob's average BER upper-bound as follows: \beqa \hat P_\ber^{\bob,\up}(R,\rho):&=& \mathbb{E} \left[ P_\ber^{\bob,\up}(R, \rho,\gamma_\bob) \right], ~~~0< \rho \leq 1 \\ &=& 0.5 \exp \left( -n  \left\{  -\ln \mathbb{E} \left[ \left( 1+ \frac{ p \gamma_\bob  }{ (1+\rho)  } \right)^{-\rho} \right] - \rho R \right\} \right) . \label{eq:avg Bob_BER_Gau}    \eeqa
The transmit power is optimized to minimize $\bar P_\ber^{\bob,\up}(R,\rho)$ subject to a security constraint constraining Eve's instantaneous BER to be greater than a threshold as follows:
\begin{subequations}
\beqa && \min_{p(\gamma_\bob, \gamma_\eve),0< \rho \leq 1,-1< \rho'<0} \hat P_\ber^{\bob,\up}(R,\rho) \\ && {\rm subject ~ to} ~   p(\gamma_\bob, \gamma_\eve) \geq 0\\ && \hspace{1.9cm} \mathbb{E}[p(\gamma_\bob, \gamma_\eve)] \leq p_\av \\ && \hspace{1.9cm}  P_\ber^{\eve,\low}(R,\rho',\gamma_\eve) \geq \calP_\ber^{\eve,\Th}.\label{eq:prob_2_opt_1_constraint_3}  \eeqa \label{eq:prob_2_opt_1}   \end{subequations}
In the following, the optimal solution is derived.

{\it Corollary 2:} The optimal solution to (\ref{eq:prob_2_opt_1}) is given by
\beq p_{\opt 2}(\gamma_\bob, \gamma_\eve) = \min \left(p_\opt^{\bob,\up}(\gamma_\bob,\hat \rho,\lambda), p_{\max}(\gamma_\eve,\tilde \rho')  \right) \label{eq:p_opt2} \eeq
where $p_{\max}(\gamma_\eve, \rho')$ is given by (\ref{eq:p_max_Eve}) and   $p_\opt^{\bob,\up}(\gamma_\bob,\rho,\lambda)$ is given by
\beq p_\opt^{\bob,\up}(\gamma_\bob,\rho,\lambda) = \left( \left(\frac{\lambda \gamma_\bob^{\rho}}{ \rho (1+  \rho)^{  \rho} }\right)^{-\frac{1}{  \rho+1}} - \frac{1+ \rho}{\gamma_\bob} \right)^+. \label{eq:p_opt_b_u} \eeq
In (\ref{eq:p_opt2}), $\tilde \rho'$ is determined by (\ref{eq:optimization_rho_prime_1}) and then $\hat \rho$ is determined by
\beqa \hat \rho &=&\arg \max_{0<\rho \leq 1}  \left( -\ln \mathbb{E} \left[ \left( 1+ \frac{ \min \left(p_\opt^{\bob,\up}(\gamma_\bob, \rho,\lambda), p_{\max}(\gamma_\eve, \tilde \rho')  \right) \gamma_\bob  }{1+\rho} \right)^{-\rho}\right] - \rho R \right) \label{eq:optimizatio_hat_rho} \eeqa where the optimal $\hat \rho$ always exists and $\lambda$ is determined such that the following condition is satisfied:\beqa \mathbb{E} [  p_{\opt 2}(\gamma_\bob, \gamma_\eve)]= p_\av . \eeqa Finally, with $p_{\opt 2}(\gamma_\bob, \gamma_\eve)$, the exponent in (\ref{eq:avg Bob_BER_Gau}) is positive: \beq -\ln \mathbb{E} \left[ \left( 1+ \frac{ p_{\opt 2}(\gamma_\bob,\gamma_\eve) \gamma_\bob  }{ (1+\hat \rho)  } \right)^{-\hat \rho} \right] - \hat \rho R>0, ~~~~ R <C_\bob. \eeq

{\it Proof of Theorem 2:} See Appendix B. \hfill $\Box$

The result of Theorem 2 can be explained as follows. If the security condition of (\ref{eq:prob_2_opt_1_constraint_3}) is {\it not} imposed, $p_\opt^{\bob,\up}(\gamma_\bob, \rho,\lambda)$ is the optimal solution to (\ref{eq:prob_2_opt_1}), which can be obtained by the Lagrangian method. Also, $p_{\max}(\gamma_\eve,\tilde \rho')$ is the maximum allowable power to avoid any security outage as discussed in Theorem 1. Therefore, the optimum power $p_{\opt 2}(\gamma_\bob,\gamma_\eve)$ must be upper-limited by $p_{\max}(\gamma_\eve,\tilde \rho')$, because the security condition of (\ref{eq:prob_2_opt_1_constraint_3}) cannot be satisfied with higher power. Overall, the the optimum power $p_{\opt 2}(\gamma_\bob,\gamma_\eve)$ is given by the minimum of $p_\opt^{\bob,\up}(\gamma_\bob, \rho,\lambda)$ and $p_{\max}(\gamma_\eve,\tilde \rho')$. Finally, $\rho$ is optimized to minimize $\bar P_\ber^{\bob,\up}(R,\rho)$ as in (\ref{eq:optimizatio_hat_rho}).

{\it Remark 5:} If we compare the two problems of (\ref{eq:prob_1_opt_1}) and (\ref{eq:prob_2_opt_1}), the security condition is instantaneously satisfied for both problems. However, the achieved BER at Bob is different for the two problems. With the optimal power allocation of Theorem 2, Bob's instantaneous BER can be higher (or lower) than the average BER upper-bound, because only the average BER upper-bound is minimized. This is in sharp contrast to the first power optimization of Theorem 1, where the data transmission is suspended if Bob's instantaneous BER is higher than a threshold, which means that Bob's instantaneous BER is guaranteed to be always higher than the threshold whenever the data is transmitted.

\subsection{numerical results}

We now evaluate Bob's average BER upper-bound $\bar P_\ber^{\bob, \up}(R, \hat \rho)$ of (\ref{eq:avg Bob_BER_Gau}) with optimal $\hat \rho$. Rate $R$ is set to 2 and the security condition is given by $\varepsilon_\ber^{\eve,\Th}=10^{-4}$. Three different blocklengths are considered: $n \in \{500, 10^3, 10^4\}$. Applying the optimal power allocation of Theorem 2, the achieved minimum $\bar P_\ber^{\bob, \up}(R, \hat \rho)$ is presented in Fig. \ref{fig:BER_minimization_opt}. As can be expected, with more power $p_{\rm av}$ or longer blocklength $n$, Bob's average BER upper-bound improves.

%\begin{figure}[h]
%\begin{center}
%\includegraphics[width=0.7\columnwidth]{figure/BER_minimization_opt}
%\caption{Bob's average BER upper-bound $\bar P_\ber^{\bob, \up}(R, \hat \rho)$ obtained by the optimal power allocation of Theorem 2. $\varepsilon_\ber^{\eve,\Th}=10^{-4}$. $\mathbb{E}[|h_\bob|^2]=2$ and $\mathbb{E}[|h_\eve|^2]=1$. $R=2$.}
%\label{fig:BER_minimization_opt}
%\end{center}
%\end{figure}

\clearpage \newpage

\section*{Appendix A\\Proof of Theorem 2}

\setcounter{equation}{0}

The problem of (\ref{eq:prob_2_opt_1}) can be rewritten as \begin{subequations} \beqa &&  \min_{0< \rho(\gamma_\bob) \leq 1, -1<\rho'(\gamma_\eve) <0} \min_{p(\gamma_\bob,\gamma_\eve,\rho(\gamma_\bob),\rho'(\gamma_\eve))} \bar P_\ber^{\bob,\up}(R) \\ && {\rm subject ~ to} ~   p(\gamma_\bob,\gamma_\eve,\rho(\gamma_\bob),\rho'(\gamma_\eve)) \geq 0\\ && \hspace{1.9cm} \mathbb{E}[p(\gamma_\bob,\gamma_\eve,\rho(\gamma_\bob),\rho'(\gamma_\eve))] \leq p_\av   \\ &&  \hspace{1.9cm}   p(\gamma_\bob,\gamma_\eve,\rho(\gamma_\bob),\rho'(\gamma_\eve)) \leq p_{\max}(\gamma_\eve,\rho') \label{eq:equivalent_optimization_2_constraint_3}   \eeqa \end{subequations}
where (\ref{eq:equivalent_optimization_2_constraint_3}) is obtained by substituting $P_\ber^{\eve,\low}(R,\rho'(\gamma_\eve),\gamma_\eve)$ of (\ref{eq:Eve_BER_Gau}) into (\ref{eq:prob_2_opt_1_constraint_3}) and $p_{\max}(\gamma_\eve,\rho')$ is given by (\ref{eq:p_max_Eve}). Using the Lagrangian multiplier, it is possible to derive the optimal solution given by \beq p_{\opt 2}(\gamma_\bob,\gamma_\eve,\rho(\gamma_\bob),\rho'(\gamma_\eve)) = \min \left(   \left( \left(\frac{\lambda \gamma_\bob^{\rho(\gamma_\bob)}}{\rho(\gamma_\bob) (1+ \rho(\gamma_\bob))^{ \rho(\gamma_\bob)} }\right)^{-\frac{1}{ \rho(\gamma_\bob)+1}} - \frac{1+\rho(\gamma_\bob)}{\gamma_\bob} \right)^+, p_{\max}(\gamma_\eve, \rho') \right) \eeq
where
$\lambda$ is determined such that the average power constraint is satisfied:
\beqa \mathbb{E} [  p_{\opt 2}(\gamma_\bob,\gamma_\eve,\rho(\gamma_\bob), \rho'(\gamma_\eve))]= p_\av.  \eeqa

We now optimize $\rho(\gamma_\bob)$ and $\rho'(\gamma_\eve)$ to minimize $\bar P_\ber^{\bob,\up}(R)$ with $p_{\opt 2}(\gamma_\bob,\gamma_\eve,\rho(\gamma_\bob),\rho'(\gamma_\eve))$ as follows:
\beqa && (\hat \rho(\gamma_\bob), \hat \rho'(\gamma_\eve)) \non \\ &=& \arg \min_{0<\rho(\gamma_\bob) \leq 1,-1< \rho'(\gamma_\eve)<0} \left.
\bar P_\ber^{\bob,\up}(R) \right|_{p=p_{\opt 2}(\gamma_\bob,\gamma_\eve, \rho(\gamma_\bob),\rho'(\gamma_\eve))}\\
&=&\arg \max_{0<\rho(\gamma_\bob) \leq 1,-1< \rho'(\gamma_\eve)<0}  \left( -\ln \left( 1+ \frac{ \min \left( p_\opt^{\bob,\up}(\gamma_\bob,\rho(\gamma_\bob),\lambda), p_{\max}(\gamma_\eve,\rho') \right) \gamma_\bob  }{1+\rho(\gamma_\bob)} \right)^{-\rho(\gamma_\bob)} - \rho(\gamma_\bob) R \right) \non \\ \\ &=&\arg \max_{0<\rho(\gamma_\bob) \leq 1}  \left( -\ln \left( 1+ \frac{ \min \left( p_\opt^{\bob,\up}(\gamma_\bob,\rho(\gamma_\bob),\lambda), \max_{-1 <\rho' <0} p_{\max}(\gamma_\eve,\rho') \right) \gamma_\bob  }{1+\rho(\gamma_\bob)  } \right)^{-\rho(\gamma_\bob)} - \rho(\gamma_\bob) R \right). \non \\ \eeqa
The optimal $\hat \rho'$ is first obtained by
\beqa \hat \rho' &=& \arg \max_{-1< \rho' <0} p_{\max}(\gamma_\eve,\rho') \\ &=& \tilde \rho'. \eeqa
Then optimal $\hat \rho(\gamma_\bob)$ is obtained by minimizing $\bar P_\ber^{\bob,\up}(R)$: \beqa \hat \rho(\gamma_\bob) &=& \arg \max_{0 < \rho(\gamma_\bob) \leq 1} \left\{ -\ln  \left( 1+ \frac{ p_{\opt 2} (\gamma_\bob,\gamma_\eve,\rho(\gamma_\bob), \tilde \rho') \gamma_\bob  }{1+\rho(\gamma_\bob)} \right)^{-\rho(\gamma_\bob)}- \rho(\gamma_\bob) R  \right\}. \label{eq:appendix_B_hat_rho} \eeqa

Finally, to show the existence of the optimal solution $\hat \rho(\gamma_\bob)$, we rewrite the term $-\ln (\cdot)$ in (\ref{eq:appendix_B_hat_rho}) as follows: \beqa -\ln  \left( 1+ \frac{ p_{\opt 2}(\gamma_\bob,\gamma_\eve,\rho, \tilde \rho') \gamma_\bob  }{1+\rho} \right)^{-\rho} &=& -\ln   \int_{y_\bob} \left[ \int_x q_{\cal CN}(x) f(y_\bob|x, h_\bob)^{\frac{1}{1+\rho}}   dx \right]^{1+\rho} dy_\bob \non \\ \\ &=:&  E_0^\bob(\rho, q_{\cal CN}(x)) \eeqa where $q_{\cal CN}(x) ={\cal CN}(0,p_\opt(\gamma_\bob,\gamma_\eve,\rho, \breve \rho'))$ and $f(y_\bob|x, h_\bob)$ is given by (\ref{eq:bob_transition_Gau}).
Following the proof of \cite[Theorem 5.6.3 ]{gallager}, it can be shown that, with $\rho >0$, we have $\bar E_0^\bob(\rho,q(x)) > 0$, $\frac{\partial}{\partial \rho}\bar E_0^\bob(\rho,q(x)) > 0$, and $\frac{\partial^2}{\partial \rho^2}\bar E_0^\bob(\rho,q(x)) \leq 0$ for $R< C_\bob$ and for any $q(x)$. The cost function $\{-\ln \mathbb{E}[\cdot]-\rho R\}$ in (\ref{eq:appendix_B_hat_rho}) is the difference between a convex function and a straight line; and thus, the cost function is convex too. Based on the proof of \cite[Theorem 5.6.3 ]{gallager}, for $R<C_\bob$ and for any $q(x)$, it can be shown that optimal $\hat \rho$ exists in $(0,1]$ and the achieved maximum value is positive: \beq \max_{0 < \rho \leq 1} \left\{ \bar E_0^\bob(\rho,q(x)) -\rho R \right\} >0, ~~~~{\rm for~} R< C_\bob {\rm ~ and ~for ~ any~} q(x). \eeq

\clearpage \newpage

\section*{Appendix B\\Proof of Corollary 2}

\setcounter{equation}{0}

The problem of (\ref{eq:prob_2_opt_1}) can be rewritten as \begin{subequations} \beqa &&  \min_{0< \rho \leq 1, -1<\rho' <0} \min_{p(\gamma_\bob,\gamma_\eve,\rho,\rho')} \bar P_\ber^{\bob,\up}(R,\rho) \\ && {\rm subject ~ to} ~   p(\gamma_\bob,\gamma_\eve,\rho,\rho') \geq 0\\ && \hspace{1.9cm} \mathbb{E}[p(\gamma_\bob,\gamma_\eve,\rho,\rho')] \leq p_\av   \\ &&  \hspace{1.9cm}   p(\gamma_\bob,\gamma_\eve,\rho,\rho') \leq p_{\max}(\gamma_\eve,\rho') \label{eq:equivalent_optimization_2_constraint_3}   \eeqa \end{subequations}
where (\ref{eq:equivalent_optimization_2_constraint_3}) is obtained by substituting $P_\ber^{\eve,\low}(R,\rho',\gamma_\eve)$ of (\ref{eq:Eve_BER_Gau}) into (\ref{eq:prob_2_opt_1_constraint_3}) and $p_{\max}(\gamma_\eve,\rho')$ is given by (\ref{eq:p_max_Eve}). Using the Lagrangian multiplier, it is possible to derive the optimal solution given by \beq p_{\opt 2}(\gamma_\bob,\gamma_\eve,\rho,\rho') = \min \left(   \left( \left(\frac{\lambda \gamma_\bob^{\rho}}{\rho (1+ \rho)^{ \rho} }\right)^{-\frac{1}{ \rho+1}} - \frac{1+\rho}{\gamma_\bob} \right)^+, p_{\max}(\gamma_\eve, \rho') \right) \eeq
where
$\lambda$ is determined such that the average power constraint is satisfied:
\beqa \mathbb{E} [  p_{\opt 2}(\gamma_\bob,\gamma_\eve,\rho, \rho')]= p_\av.  \eeqa

We now optimize $\rho$ and $\rho'$ to minimize $\bar P_\ber^{\bob,\up}(R,\rho)$ with $p_{\opt 2}(\gamma_\bob,\gamma_\eve,\rho,\rho')$ as follows:
\beqa && (\hat \rho, \hat \rho') \non \\ &=& \arg \min_{0<\rho \leq 1,-1< \rho'<0} \left.
\bar P_\ber^{\bob,\up}(R) \right|_{p=p_{\opt 2}(\gamma_\bob,\gamma_\eve, \rho,\rho')}\\
&=&\arg \max_{0<\rho \leq 1,-1< \rho'<0}  \left( -\ln \mathbb{E} \left[ \left( 1+ \frac{ \min \left( p_\opt^{\bob,\up}(\gamma_\bob,\rho,\lambda), p_{\max}(\gamma_\eve,\rho') \right) \gamma_\bob  }{1+\rho} \right)^{-\rho}\right] - \rho R \right) \non \\ \\ &=&\arg \max_{0<\rho \leq 1}  \left( -\ln \mathbb{E} \left[ \left( 1+ \frac{ \min \left( p_\opt^{\bob,\up}(\gamma_\bob,\rho,\lambda), \max_{-1 <\rho' <0} p_{\max}(\gamma_\eve,\rho') \right) \gamma_\bob  }{1+\rho  } \right)^{-\rho}\right] - \rho R \right). \non \\ \eeqa
The optimal $\hat \rho'$ is first obtained by
\beqa \hat \rho' &=& \arg \max_{-1< \rho' <0} p_{\max}(\gamma_\eve,\rho') \\ &=& \tilde \rho'. \eeqa
Then optimal $\hat \rho$ is obtained by minimizing $\bar P_\ber^{\bob,\up}(R)$: \beqa \hat \rho &=& \arg \max_{0 < \rho \leq 1} \left\{ -\ln \mathbb{E} \left[ \left( 1+ \frac{ p_{\opt 2} (\gamma_\bob,\gamma_\eve,\rho, \tilde \rho') \gamma_\bob  }{1+\rho} \right)^{-\rho}\right]- \rho R  \right\}. \label{eq:appendix_B_hat_rho} \eeqa

Finally, to show the existence of the optimal solution $\hat \rho$, we rewrite the term $-\ln \mathbb{E}[\cdot]$ in (\ref{eq:appendix_B_hat_rho}) as follows: \beqa -\ln \mathbb{E} \left[ \left( 1+ \frac{ p_{\opt 2}(\gamma_\bob,\gamma_\eve,\rho, \tilde \rho') \gamma_\bob  }{1+\rho} \right)^{-\rho}\right] &=& -\ln \mathbb{E}\left[  \int_{y_\bob} \left[ \int_x q_{\cal CN}(x) f(y_\bob|x, h_\bob)^{\frac{1}{1+\rho}}   dx \right]^{1+\rho} dy_\bob \right]\non \\ \\ &=:& \bar E_0^\bob(\rho, q_{\cal CN}(x)) \eeqa where $q_{\cal CN}(x) ={\cal CN}(0,p_\opt(\gamma_\bob,\gamma_\eve,\rho, \breve \rho'))$ and $f(y_\bob|x, h_\bob)$ is given by (\ref{eq:bob_transition_Gau}).
Following the proof of \cite[Theorem 5.6.3 ]{gallager}, it can be shown that, with $\rho >0$, we have $\bar E_0^\bob(\rho,q(x)) > 0$, $\frac{\partial}{\partial \rho}\bar E_0^\bob(\rho,q(x)) > 0$, and $\frac{\partial^2}{\partial \rho^2}\bar E_0^\bob(\rho,q(x)) \leq 0$ for $R< C_\bob$ and for any $q(x)$. The cost function $\{-\ln \mathbb{E}[\cdot]-\rho R\}$ in (\ref{eq:appendix_B_hat_rho}) is the difference between a convex function and a straight line; and thus, the cost function is convex too. Based on the proof of \cite[Theorem 5.6.3 ]{gallager}, for $R<C_\bob$ and for any $q(x)$, it can be shown that optimal $\hat \rho$ exists in $(0,1]$ and the achieved maximum value is positive: \beq \max_{0 < \rho \leq 1} \left\{ \bar E_0^\bob(\rho,q(x)) -\rho R \right\} >0, ~~~~{\rm for~} R< C_\bob {\rm ~ and ~for ~ any~} q(x). \eeq

{\it Temp 1:} Take expectation $\mathbb{E}[\cdot]$ to both sides of \cite[eq. (5B.11)]{gallager} and then take logarithm as in eq. (5B.12).

{\it Temp 2:}Following the approach \cite{Arimoto}, \cite[Lemma 3.2.1]{viterbi}, it can be shown that, with $-1< \rho' <0$, we have $\bar E_0^\eve(\rho',q(x)) < 0$, $\frac{\partial}{\partial \rho'}\bar E_0^\eve(\rho',q(x)) > 0$, and $\frac{\partial^2}{\partial \rho'^2}\bar E_0^\eve(\rho',q(x)) \leq 0$ for $R> C_\eve$ and any $q(x)$. Then it can be shown that optimal $\tilde \rho'$ exists in $(-1,0)$ and the achieved maximum value is positive as follows: \beqa 0 & < & \max_{-1 < \rho' <0} \left\{ \min_{q(x)} \bar E_0^\eve(\rho',q(x)) -\rho' R \right\} , ~~~~ R >  C_\eve \\ & \leq & \max_{-1 < \rho' <0} \left\{  \bar E_0^\eve(\rho',q_{\cal CN}(x)) -\rho' R \right\} , ~~~~ R >  C_\eve \eeqa where the inequality is due to \cite{Arimoto}, \cite[Theorem 3.9.1]{viterbi}.

%%%
